# Supplementary material for: Micromagnet-free operation of electron spin qubits in Si/Si$_{1-x}$Ge$_x$ vertical double quantum dots
Source: arXiv:2512.19785 source file (2025-12-22)
Supplement: Supplementary file 1 [file SiSiGevDQD_suppl.pdf]

# Supplementary Material: Micromagnet-free operation of electron spin qubits in $Si/Si_{1-x}Ge_x$ vertical double quantum dots

Abhikbrata Sarkar[1] and Daniel Loss[1, 2, 3, 4]

[1] *Department of Physics, University of Basel, Klingelbergstrasse 82, 4056 Basel, Switzerland*
[2] *Physics Department, King Fahd University of Petroleum and Minerals, 31261, Dhahran, Saudi Arabia*
[3] *Center for Advanced Quantum Computing, KFUPM, Dhahran, Saudi Arabia*
[4] *RDIA Chair in Quantum Computing*

(Dated: December 21, 2025)

### Geometry-dependency: valley splitting, shear strain and electrical tunability in the vertical DQD

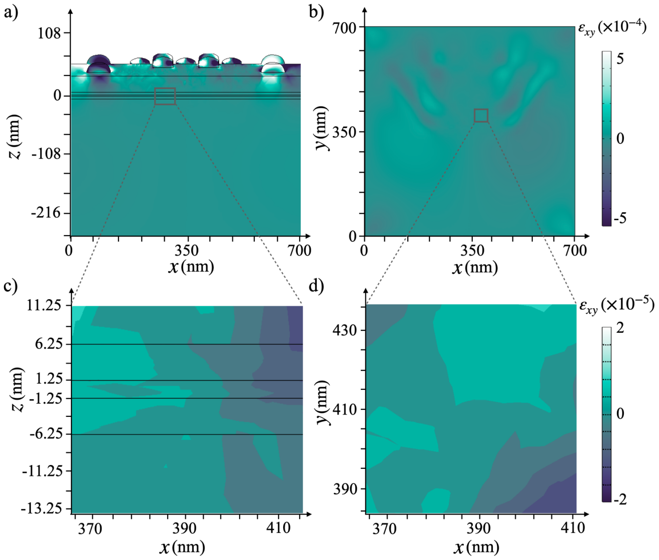


FIG. S1. **Simulated shear strain in the DQD due to the metal gate electrodes atop the $Si/Si_{1-x}Ge_x$ heterostructure.** a) The $xz$-map of the $\varepsilon_{xy}(x, y, z)$ shear strain tensor component in the simulated DQD device. b) Similarly, the $xy$-map of $\varepsilon_{xy}(x, y, z)$. c-d) The 2D maps of $\varepsilon_{xy}(x, y, z)$ in the DQD under plunger gate $P_1$. The $Si/Si_{1-x}Ge_x/Si$ ($x$=0.033 here) layers are indicated in c). The DQD centered at point $(390, 410, 0)$ nm spans the following range: $x\in[370, 410]$ nm, $y\in[390, 430]$ nm, $z\in[-6.25, 6.25]$ nm.

3D finite element method (FEM) simulations of the strain distribution at 0.1 K are performed using the Structural Mechanics module in COMSOL Multiphysics. The metal gate electrodes are modeled as stress-inducing layers on top of the $Si/Si_{1-x}Ge_x$ heterostructure, and the resulting strain tensor is evaluated throughout the DQD region (Fig. S1). Standard material parameters for Si and $Si_{1-x}Ge_x$ from literature have been used [1, 2]. Few of the relevant $Si_{1-x}Ge_x$ parameters are listed in Tab. S1.

The dominant contribution to the large valley splitting originates from coherent interference of intervalley coupling at the two Si/SiGe interfaces defining the vertical double well. We first examine the dependence of the valley splitting on the barrier height, set by the Ge concentration $x$ in the $Si_{1-x}Ge_x$ barrier. Varying $x$ from 1.1% to 5.5%, we find that for $V_b$=15 meV, corresponding to $x$=3.3% ($Si_{0.967}Ge_{0.033}$), the valley splitting is maximized (Fig. S2a). In the absence of shear strain, varying the barrier width $a$ between 2 and 3 nm yields oscillations in the valley splitting ranging from 260 $\mu$eV down to 25 $\mu$eV. When realistic gate-induced shear strain is included, these oscillations are substantially modified, with the valley splitting varying between 275 $\mu$eV and 90 $\mu$eV (Fig. S2b). Furthermore, at finite plunger fields $|F_z| > 0$, the oscillations are suppressed and a uniformly large valley splitting of order 150 $\mu$eV emerges (Fig. S2c). This behavior reflects the interference of interface-induced intervalley coupling contributions from the two barrier interfaces. Since $2k_0 \approx 9.5$ nm$^{-1}$, the relative phase of these contributions is sensitive to changes in the barrier width on the scale of a monolayer ($\sim$ 0.14 nm). Consistently, we find that the valley splitting exhibits peak-to-peak oscillations when $a$ is varied by approximately 0.16 nm. Gate-induced strain breaks the symmetry between the two interfaces, modifying the relative weighting of their contributions and thereby elevating the minimum valley splitting to 90 $\mu$eV. Importantly, while the valley splitting exhibits oscillations on the monolayer scale at zero plunger field, gate-induced strain in realistic devices and plunger field strongly suppress this sensitivity, yielding a robust lower bound $\sim$150 $\mu$eV that is insensitive to atomic scale variations in barrier thickness. We also examine the effect of varying the barrier height on the electrical tun-

| paramaters | values |
|---|---|
| lattice constant, $a_l$ | $(5.43{+}0.20x{+}0.03x^2){\times}10^{-10}$ m |
| density, $\rho$ | $(2.3{+}3.5x{-}0.5x^2){\times}10^3$ g cm$^{-3}$ |
| Young's modulus, $E$ | $(130.2 - 28.1x){\times}10^9$ Pa |
| thermal expansion coeff.,$\alpha$ | $(2.60 + 2.55x){\times}10^{-6}$ K$^{-1}$ |
| heat capacity, $C_p$ | $\frac{19.6+2.9x}{72.6x+28.1(1-x)}{\times}10^3$ J Kg$^{-1}$K$^{-1}$ |
| band gap, $E_g$ | $1.12 - 0.41x + 0.008x^2$ eV |
| Poisson's ratio, $\nu$ | $0.278 - 0.005x$ |
| relative permittivity, $\varepsilon_r$ | $11.7 + 4.5x$ |

TABLE S1. **$Si_{1-x}Ge_x$ parameters as a function of Ge fraction $x$.** For $x$=0, these parameters correspond to Si. Note that the value of thermal conductivity $K$ has been taken from the plot in Ref. [2] highlighting its nontrivial variation with $x$.

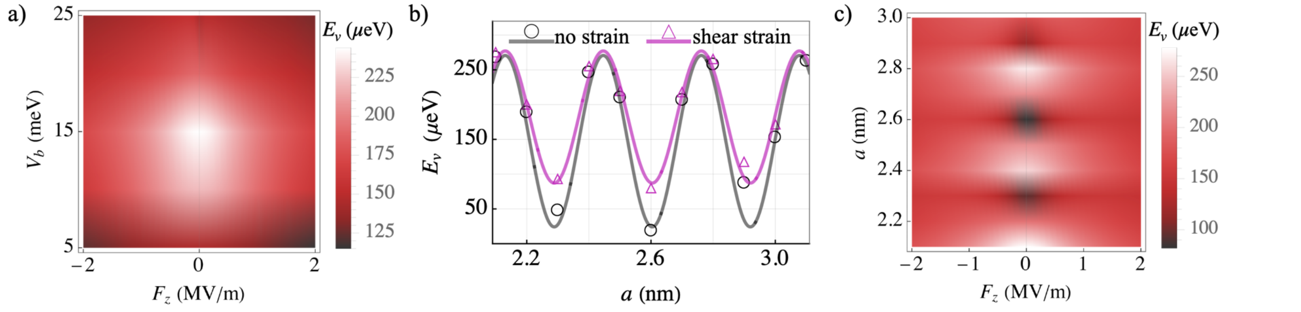


FIG. S2. **Valley Splitting dependence on barrier height and width.** a) 2D map of the valley splitting $E_v$ as a function of plunger voltage $F_z$ and $Si_{1-x}Ge_x$ barrier height $V_b$. $V_b$=15 ($x$=3.3%) exhibits the largest valley splitting. b) Valley splitting $E_v$ as a function of the barrier width $a$ at $F_z$=0. The circles and solid fit line in black denote the results without strain; while triangular markers and solid fit line in purple show results with strain. The oscillation in the valley splitting can be fit to a period of 0.31 nm. c) 2D map of $E_v$ as a function of $F_z$ and barrier width $a$ in the presence of gate-induced shear strain.

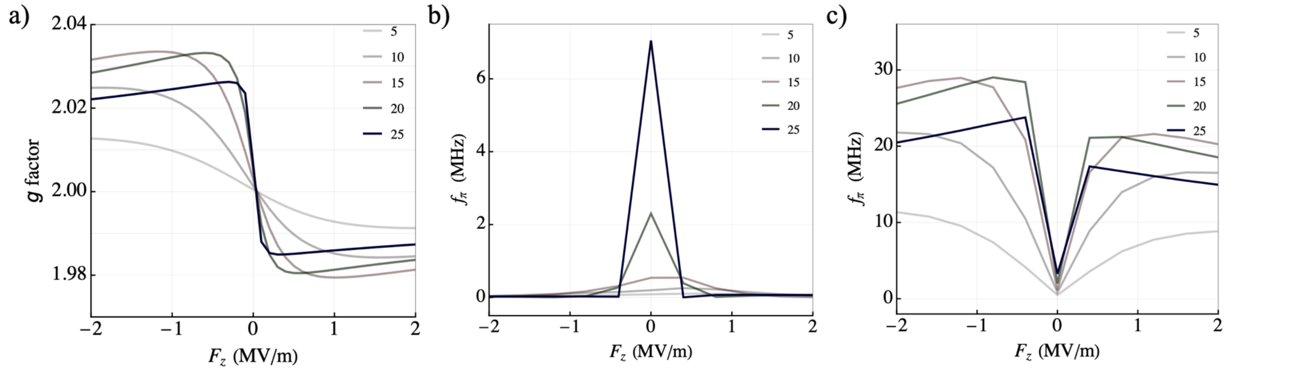


FIG. S3. **Electrical tunability with varying barrier height.** a) $g$ factor as a function of plunger voltage $F_z$ for different $Si_{1-x}Ge_x$ barrier heights $V_b$ (plot legends given in meV). b) EDSR Rabi frequency $f_\pi$ as a function of $F_z$ at different barrier heights $V_b$; $\mathbf{B}\|\hat{\mathbf{x}}$,$\mathbf{E}_{\rm ac}\|\hat{\mathbf{z}}$. c) $f_\pi$ vs. $F_z$ at different barrier heights $V_b$; $\mathbf{B}\|\hat{\mathbf{x}}$,$\mathbf{E}_{\rm ac}\|\hat{\mathbf{x}}$. The barrier width is $a$=2.5 nm.

ability of the electron spin qubit. With increasing barrier height, the slope of the $g$ factor increases, while $V_b$=15 meV ($x$=3.3%) produces the largest variation (Fig. S3a). As anticipated, the EDSR Rabi frequency for microwave drive via the plunger gate enhances with increasing maximum $\frac{\partial g}{\partial F_z}$ close to $F_z$=0 (Fig. S3b). EDSR with in-plane ac electric field ($\mathbf{E}_{\rm ac}\|\ \hat{\mathbf{x}}$) is the fastest for $V_b$=15, close to plunger field value where $\frac{\partial g}{\partial F_z} \approx 0$ (Fig. S3).

### The z-double well potential basis

The double well potential is given by,

$$V(\mathbf{r}) = V_{\rm DW}(z) + \frac{m_t}{2}\left(\left[\frac{\hbar}{m_t L_x^2}\right]^2 x^2 + \left[\frac{\hbar}{m_t L_y^2}\right]^2 y^2\right). \quad (1)$$

The $z$-basis states are calculated by solving the following equation: $\left[-\frac{\hbar^2\partial_z^2}{2m_l} + V_{\rm DW}\right]\phi_n(z) = e_n\phi_n(z)$. The piecewise function describing the double well potential is as follows:

$$V_{\rm DW}(z,a,L,V_b) = \begin{cases} V_0 & L+\frac{a}{2} \leq z < \infty \\ 0 & \frac{a}{2} < z < L+\frac{a}{2} \\ V_b & -\frac{a}{2} \leq z \leq \frac{a}{2} \\ 0 & -\left(L+\frac{a}{2}\right) < z < -\frac{a}{2} \\ V_0 & -\infty < z \leq -\left(L+\frac{a}{2}\right). \end{cases} \quad (2)$$

Below, we provide the full form of the transcendental equation and basis solutions for even and odd bound ($e_n < V_b$) and unbound ($e_n > V_b$) states. Note that $\gamma = \sqrt{\frac{2mL^2V_b}{\hbar^2}}$, $r = \frac{a}{2L}$.

For $\mathbf{e_n} < \mathbf{V_b}$, **even**:

$$\gamma\pi\sqrt{\frac{e_n}{V_b}}(1+r)=n\pi+\tan^{-1}\left[-F\frac{1+\frac{e_n}{F\sqrt{V_0^2-e_n^2}}}{1-\frac{e_nF}{\sqrt{V_0^2-e_n^2}}}\right],$$

$$\text{where,}\quad F=\frac{\cos\left(\gamma\sqrt{\frac{e_n}{V_b}}\pi r\right)\cosh\left(\gamma\sqrt{1-\frac{e_n}{V_b}}\pi r\right)-\sqrt{\frac{V_b}{e_n}-1}\sin\left(\gamma\sqrt{\frac{e_n}{V_b}}\pi r\right)\sinh\left(\gamma\sqrt{1-\frac{e_n}{V_b}}\pi r\right)}{\sin\left(\gamma\sqrt{\frac{e_n}{V_b}}\pi r\right)\cosh\left(\gamma\sqrt{1-\frac{e_n}{V_b}}\pi r\right)+\sqrt{\frac{V_b}{e_n}-1}\cos\left(\gamma\sqrt{\frac{e_n}{V_b}}\pi r\right)\sinh\left(\gamma\sqrt{1-\frac{e_n}{V_b}}\pi r\right)}, \tag{3}$$

$$\phi_n(z)=\mathbf{N}\times\begin{cases}\dfrac{\mathbf{num}(F)\cos\left(\gamma\sqrt{\frac{e_n}{V_b}}\pi(1+r)\right)+\mathbf{den}(F)\sin\left(\gamma\sqrt{\frac{e_n}{V_b}}\pi(1+r)\right)}{e^{-\gamma V_b^{-1}\sqrt{V_0^2-e_n^2}\pi(1+r)}}e^{\gamma V_b^{-1}\sqrt{V_0^2-e_n^2}\pi z/L}, & -\infty<z\le -L(1+r)\\ \mathbf{num}(F)\cos\left(-\gamma\sqrt{\frac{e_n}{V_b}}\pi\frac{z}{L}\right)+\mathbf{den}(F)\sin\left(-\gamma\sqrt{\frac{e_n}{V_b}}\pi\frac{z}{L}\right), & -L(1+r)<z<-Lr\\ \cosh\left(\gamma\sqrt{1-\frac{e_n}{V_b}}\pi\frac{z}{L}\right), & -Lr\le z\le Lr\\ \mathbf{num}(F)\cos\left(\gamma\sqrt{\frac{e_n}{V_b}}\pi\frac{z}{L}\right)+\mathbf{den}(F)\sin\left(\gamma\sqrt{\frac{e_n}{V_b}}\pi\frac{z}{L}\right), & Lr<z<L(1+r)\\ \dfrac{\mathbf{num}(F)\cos\left(\gamma\sqrt{\frac{e_n}{V_b}}\pi(1+r)\right)+\mathbf{den}(F)\sin\left(\gamma\sqrt{\frac{e_n}{V_b}}\pi(1+r)\right)}{e^{-\gamma V_b^{-1}\sqrt{V_0^2-e_n^2}\pi(1+r)}}e^{-\gamma V_b^{-1}\sqrt{V_0^2-e_n^2}\pi z/L}, & -\infty<z\le -L(1+r),\end{cases} \tag{4}$$

For $\mathbf{e_n}<\mathbf{V_b}$, **odd**:

$$\gamma\pi\sqrt{\frac{e_n}{V_b}}(1+r)=n\pi+\tan^{-1}\left[-F\frac{1+\frac{e_n}{F\sqrt{V_0^2-e_n^2}}}{1-\frac{e_nF}{\sqrt{V_0^2-e_n^2}}}\right],$$

$$\text{where,}\quad F=\frac{\cos\left(\gamma\sqrt{\frac{e_n}{V_b}}\pi r\right)\sinh\left(\gamma\sqrt{1-\frac{e_n}{V_b}}\pi r\right)-\sqrt{\frac{V_b}{e_n}-1}\sin\left(\gamma\sqrt{\frac{e_n}{V_b}}\pi r\right)\cosh\left(\gamma\sqrt{1-\frac{e_n}{V_b}}\pi r\right)}{\sin\left(\gamma\sqrt{\frac{e_n}{V_b}}\pi r\right)\sinh\left(\gamma\sqrt{1-\frac{e_n}{V_b}}\pi r\right)+\sqrt{\frac{V_b}{e_n}-1}\cos\left(\gamma\sqrt{\frac{e_n}{V_b}}\pi r\right)\cosh\left(\gamma\sqrt{1-\frac{e_n}{V_b}}\pi r\right)},$$

$$\phi_n(z)=\mathbf{N}\times\begin{cases}-\dfrac{\mathbf{num}(F)\cos\left(\gamma\sqrt{\frac{e_n}{V_b}}\pi(1+r)\right)+\mathbf{den}(F)\sin\left(\gamma\sqrt{\frac{e_n}{V_b}}\pi(1+r)\right)}{e^{-\gamma V_b^{-1}\sqrt{V_0^2-e_n^2}\pi(1+r)}}e^{\gamma V_b^{-1}\sqrt{V_0^2-e_n^2}\pi z/L}, & -\infty<z\le -L(1+r)\\ -\mathbf{num}(F)\cos\left(-\gamma\sqrt{\frac{e_n}{V_b}}\pi\frac{z}{L}\right)-\mathbf{den}(F)\sin\left(-\gamma\sqrt{\frac{e_n}{V_b}}\pi\frac{z}{L}\right), & -L(1+r)<z<-Lr\\ \sinh\left(\gamma\sqrt{1-\frac{e_n}{V_b}}\pi\frac{z}{L}\right), & -Lr\le z\le Lr\\ \mathbf{num}(F)\cos\left(\gamma\sqrt{\frac{e_n}{V_b}}\pi\frac{z}{L}\right)+\mathbf{den}(F)\sin\left(\gamma\sqrt{\frac{e_n}{V_b}}\pi\frac{z}{L}\right), & Lr<z<L(1+r)\\ \dfrac{\mathbf{num}(F)\cos\left(\gamma\sqrt{\frac{e_n}{V_b}}\pi(1+r)\right)+\mathbf{den}(F)\sin\left(\gamma\sqrt{\frac{e_n}{V_b}}\pi(1+r)\right)}{e^{-\gamma V_b^{-1}\sqrt{V_0^2-e_n^2}\pi(1+r)}}e^{-\gamma V_b^{-1}\sqrt{V_0^2-e_n^2}\pi z/L}, & -\infty<z\le -L(1+r),\end{cases} \tag{5}$$

For $\mathbf{e_n}>\mathbf{V_b}$, **even**:

$$\gamma\pi\sqrt{\frac{e_n}{V_b}}(1{+}r){=}n\pi{+}\tan^{-1}\Bigg[-F\frac{1{+}\frac{e_n}{F\sqrt{V_0^2-e_n^2}}}{1{-}\frac{e_nF}{\sqrt{V_0^2-e_n^2}}}\Bigg],$$

$$\text{where,}\quad F{=}\frac{\cos\left(\gamma\sqrt{\frac{e_n}{V_b}}\pi r\right)\cos\left(\gamma\sqrt{\frac{e_n}{V_b}-1}\pi r\right){+}\sqrt{1{-}\frac{V_b}{e_n}}\sin\left(\gamma\sqrt{\frac{e_n}{V_b}}\pi r\right)\sin\left(\gamma\sqrt{\frac{e_n}{V_b}-1}\pi r\right)}{\sin\left(\gamma\sqrt{\frac{e_n}{V_b}}\pi r\right)\cos\left(\gamma\sqrt{\frac{e_n}{V_b}-1}\pi r\right){-}\sqrt{1{-}\frac{V_b}{e_n}}\cos\left(\gamma\sqrt{\frac{e_n}{V_b}}\pi r\right)\sin\left(\gamma\sqrt{\frac{e_n}{V_b}-1}\pi r\right)},\tag{6}$$

$$\phi_n(z)=\mathbf{N}\times\begin{cases}\dfrac{\mathbf{num}(F)\cos\left(\gamma\sqrt{\frac{e_n}{V_b}}\pi(1{+}r)\right){+}\mathbf{den}(F)\sin\left(\gamma\sqrt{\frac{e_n}{V_b}}\pi(1{+}r)\right)}{e^{-\gamma V_b^{-1}\sqrt{V_0^2-e_n^2}\pi(1+r)}}e^{\gamma V_b^{-1}\sqrt{V_0^2-e_n^2}\pi z/L}, & -\infty<z\le -L\big(1+r\big)\\ \mathbf{num}(F)\cos\left(-\gamma\sqrt{\frac{e_n}{V_b}}\pi\frac{z}{L}\right)+\mathbf{den}(F)\sin\left(-\gamma\sqrt{\frac{e_n}{V_b}}\pi\frac{z}{L}\right), & -L(1+r)<z<-Lr\\ \cos\left(\gamma\sqrt{\frac{e_n}{V_b}-1}\pi\frac{z}{L}\right), & -Lr\le z\le Lr\\ \mathbf{num}(F)\cos\left(\gamma\sqrt{\frac{e_n}{V_b}}\pi\frac{z}{L}\right)+\mathbf{den}(F)\sin\left(\gamma\sqrt{\frac{e_n}{V_b}}\pi\frac{z}{L}\right), & Lr<z<L(1+r)\\ \dfrac{\mathbf{num}(F)\cos\left(\gamma\sqrt{\frac{e_n}{V_b}}\pi(1{+}r)\right){+}\mathbf{den}(F)\sin\left(\gamma\sqrt{\frac{e_n}{V_b}}\pi(1{+}r)\right)}{e^{-\gamma V_b^{-1}\sqrt{V_0^2-e_n^2}\pi(1+r)}}e^{-\gamma V_b^{-1}\sqrt{V_0^2-e_n^2}\pi z/L}, & -\infty<z\le -L\big(1+r\big),\end{cases}\tag{7}$$

For $\mathbf{e_n}>\mathbf{V_b}$, **odd**:

$$\gamma\pi\sqrt{\frac{e_n}{V_b}}(1{+}r){=}n\pi{+}\tan^{-1}\Bigg[-F\frac{1{+}\frac{e_n}{F\sqrt{V_0^2-e_n^2}}}{1{-}\frac{e_nF}{\sqrt{V_0^2-e_n^2}}}\Bigg],$$

$$\text{where,}\quad F{=}\frac{\cos\left(\gamma\sqrt{\frac{e_n}{V_b}}\pi r\right)\sin\left(\gamma\sqrt{\frac{e_n}{V_b}-1}\pi r\right){-}\sqrt{1{-}\frac{V_b}{e_n}}\sin\left(\gamma\sqrt{\frac{e_n}{V_b}}\pi r\right)\cos\left(\gamma\sqrt{\frac{e_n}{V_b}-1}\pi r\right)}{\sin\left(\gamma\sqrt{\frac{e_n}{V_b}}\pi r\right)\sin\left(\gamma\sqrt{\frac{e_n}{V_b}-1}\pi r\right){+}\sqrt{1{-}\frac{V_b}{e_n}}\cos\left(\gamma\sqrt{\frac{e_n}{V_b}}\pi r\right)\cos\left(\gamma\sqrt{\frac{e_n}{V_b}-1}\pi r\right)},$$

$$\phi_n(z)=\mathbf{N}\times\begin{cases}-\dfrac{\mathbf{num}(F)\cos\left(\gamma\sqrt{\frac{e_n}{V_b}}\pi(1{+}r)\right){+}\mathbf{den}(F)\sin\left(\gamma\sqrt{\frac{e_n}{V_b}}\pi(1{+}r)\right)}{e^{-\gamma V_b^{-1}\sqrt{V_0^2-e_n^2}\pi(1+r)}}e^{\gamma V_b^{-1}\sqrt{V_0^2-e_n^2}\pi z/L}, & -\infty<z\le -L\big(1+r\big)\\ -\mathbf{num}(F)\cos\left(-\gamma\sqrt{\frac{e_n}{V_b}}\pi\frac{z}{L}\right)-\mathbf{den}(F)\sin\left(-\gamma\sqrt{\frac{e_n}{V_b}}\pi\frac{z}{L}\right), & -L(1+r)<z<-Lr\\ \sin\left(\gamma\sqrt{\frac{e_n}{V_b}-1}\pi\frac{z}{L}\right), & -Lr\le z\le Lr\\ \mathbf{num}(F)\cos\left(\gamma\sqrt{\frac{e_n}{V_b}}\pi\frac{z}{L}\right)+\mathbf{den}(F)\sin\left(\gamma\sqrt{\frac{e_n}{V_b}}\pi\frac{z}{L}\right), & Lr<z<L(1+r)\\ \dfrac{\mathbf{num}(F)\cos\left(\gamma\sqrt{\frac{e_n}{V_b}}\pi(1{+}r)\right){+}\mathbf{den}(F)\sin\left(\gamma\sqrt{\frac{e_n}{V_b}}\pi(1{+}r)\right)}{e^{-\gamma V_b^{-1}\sqrt{V_0^2-e_n^2}\pi(1+r)}}e^{-\gamma V_b^{-1}\sqrt{V_0^2-e_n^2}\pi z/L}, & -\infty<z\le -L\big(1+r\big).\end{cases}\tag{8}$$

The transcendental equation can be solved on a graph by plotting the LHS and RHS and identifying the intersecting points to produce $e_n$ solutions for each case. The normalization coefficient $N$ can be obtained by using $\int_{-\infty}^{\infty}|\phi_n(z)|^2dz = 1$. Also, **num**() and **den**() denote the numerator and denominator of the expression in parentheses, respectively. For this work, we approximate $V_0 >> e_n$ (the infinite outer boundary of the double well), in which case $\frac{1+\frac{e_n}{F\sqrt{V_0^2-e_n^2}}}{1-\frac{e_nF}{\sqrt{V_0^2-e_n^2}}}\approx 1$.

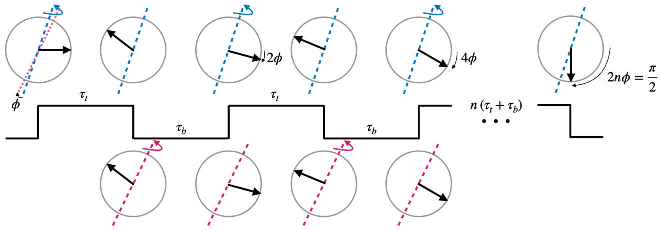


FIG. S4. **Schematic of the pulsing sequence of hopping between top and bottom Si dots.** The in-plane principle axis of the $g$ tensor are denoted in blue (red) for the top (bottom) QD, with an angular difference $\phi$ between them. Each $(\tau_t + \tau_b)$ sequence of hopping back and forth generates $2\phi$ net rotation of the spin. Hence after $n$ such sequences, e.g. single qubit $S$ gate ($\pi/2$ rotation) can be achieved if $2n\phi = \pi/2$.

The $x - y$ basis is described by the following set of equations:

$$\phi_l(x) = \frac{1}{\sqrt{2^l l!\, L_x \sqrt{\pi}}} e^{-\frac{x^2}{2L_x^2}} H_l(x/L_x)$$
$$\phi_m(y) = \frac{1}{\sqrt{2^m m!\, L_y \sqrt{\pi}}} e^{-\frac{y^2}{2L_y^2}} H_m(y/L_y). \quad (9)$$

### Hopping-based spin rotation mechanism

An anisotropic $g$ tensor can be harnessed to realize single qubit rotations via a spin hopping (or shuttling) sequence between the top and bottom dots of the DQD structure. As demonstrated in figure S4, the spin could be initialized in the top QD in the direction of the applied magnetic field $\mathbf{B} \parallel \mathbf{x}$. The spin is allowed to precess from $-\pi/2$ to $\pi/2$ about the principal $g$-tensor axis for $\tau_t$ time, followed by the spin hopping to the bottom QD. The spin then precesses from $-\pi/2$ to $\pi/2$ about the principal $g$-tensor axis of the bottom QD for $\tau_b$ time. When shuttled back to the top QD, the angular difference $\phi$ between the two $g$-tensor axes would produce a $2\phi$ rotation of the original spin orientation $\parallel \mathbf{x}$. By repeating this pulsing sequence $n$ times, a $\pi/2$ rotation of the spin about the $z$-axis, for example, can be achieved if $2n\phi = \pi/2$. The gate-time for this rotation is estimated as $T_g^{\pi/2} = \frac{n}{f_L}$, where $f_L = \frac{g\mu_B B}{h}$ is the Larmor frequency of the electron spin qubit ($f_L \simeq 2.8$ GHz for the electron spin at $|\mathbf{B}| = 100$ mT).


[1] F. Schäffler, Semiconductor Science and Technology **12**, 1515 (1997).

[2] Ioffe Institute, "SiGe: Basic properties and material parameters," https://www.ioffe.ru/SVA/NSM/Semicond/SiGe/basic.html.
